# Supplementary material for: Tangent: An Empirical Study of Testing Practices for LLM-Based Agent Applications
Source: arXiv:2608.08413 source file (2026-08-09)
Supplement: Supplementary file 1 [file supplementary.tex]

\begin{figure}
    \centering
    \includegraphics[width=\linewidth]{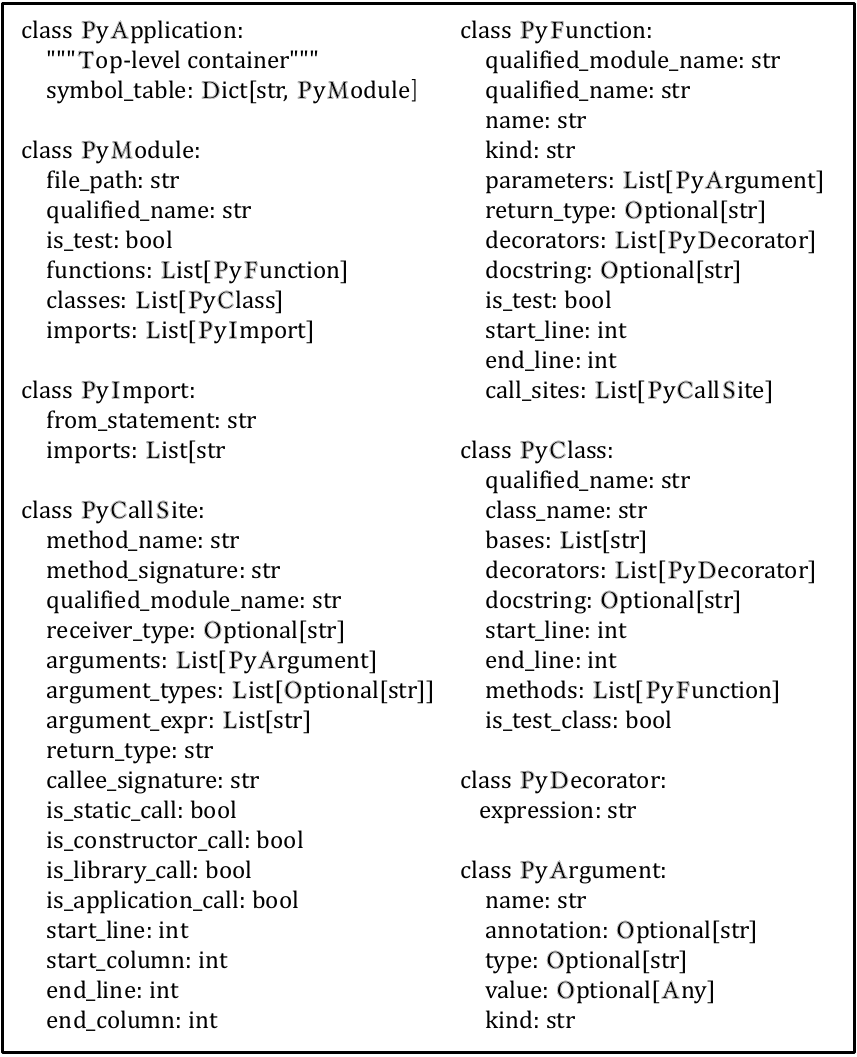}
    \caption{The \beaver code analysis model.}
    \label{fig:codemodel}
\end{figure}


\begin{figure}[t]
    \centering
    \includegraphics[width=\linewidth]{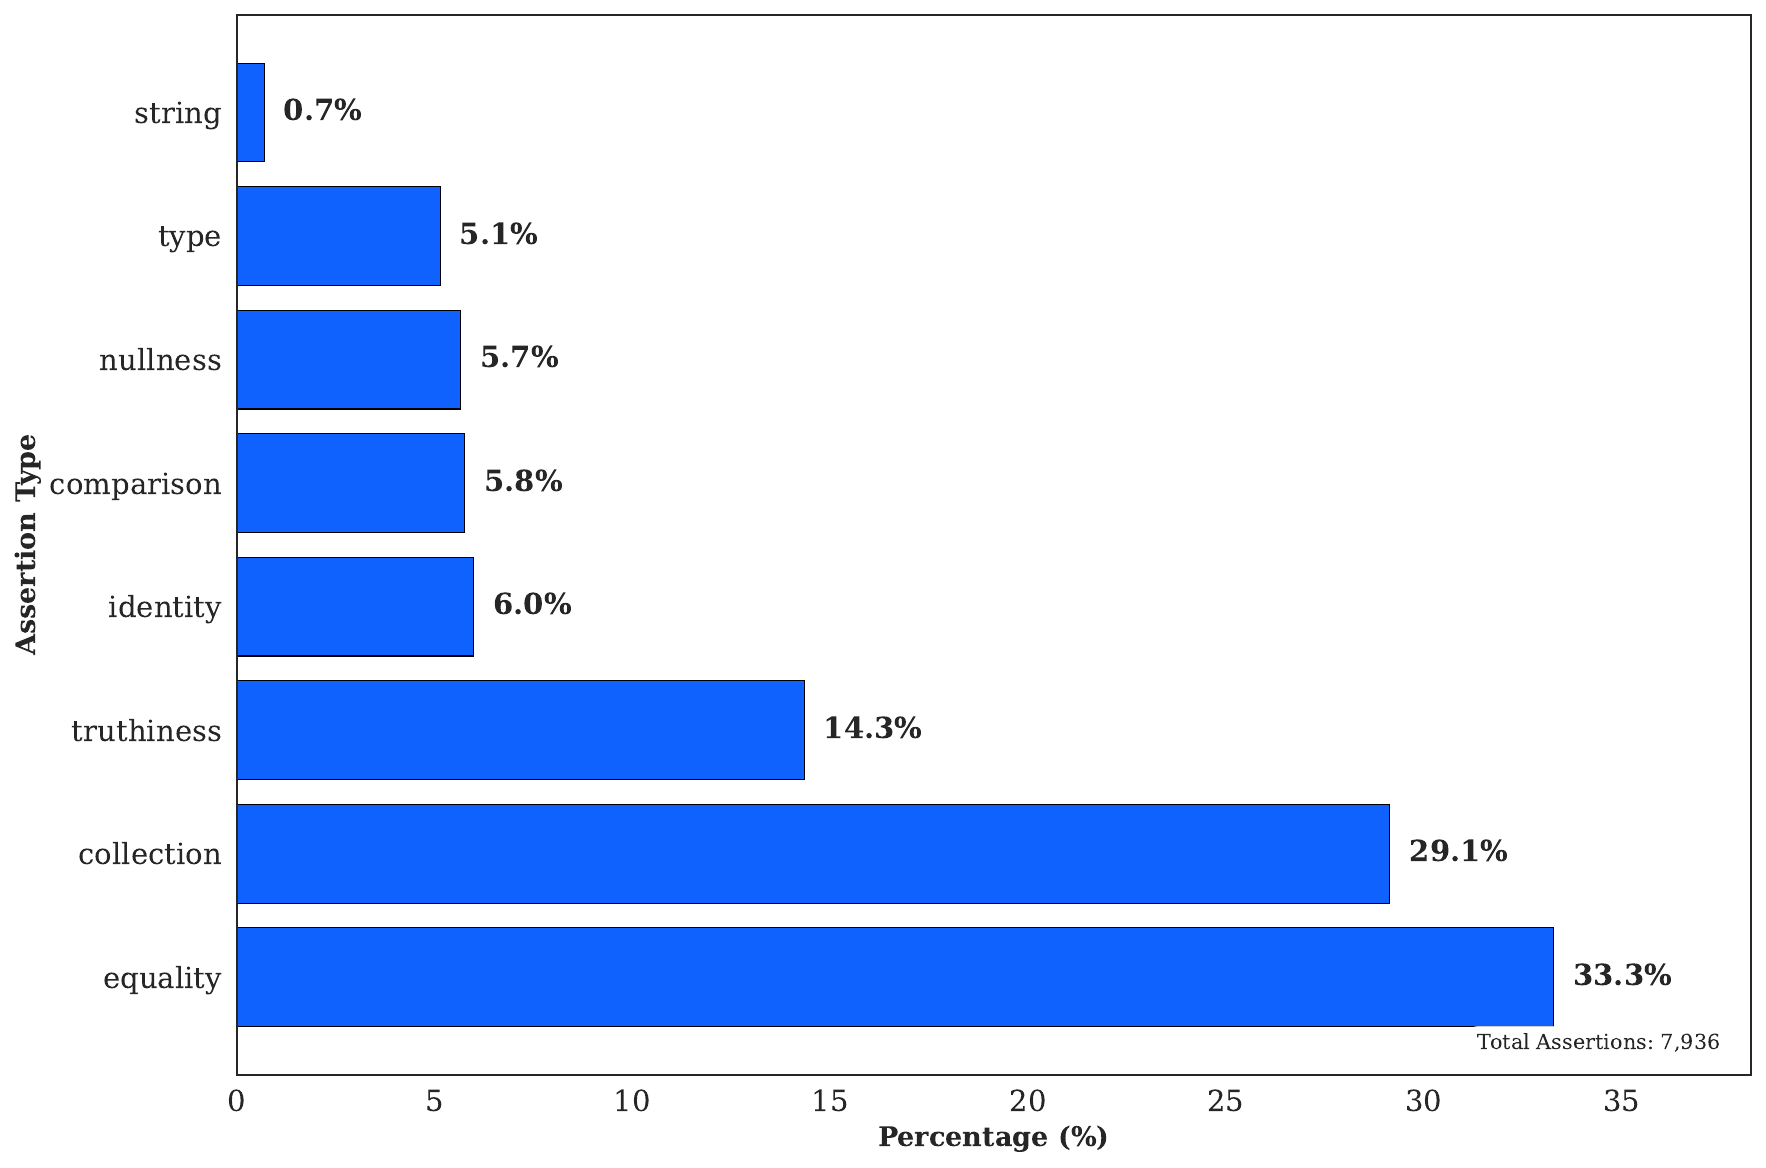}
    \caption{Distribution of assertion types.}
    \label{fig:assertion_type}
\end{figure}

\input{rq5_agent_test_complexity}
\begin{figure}
    \centering
    \includegraphics[width=\linewidth]{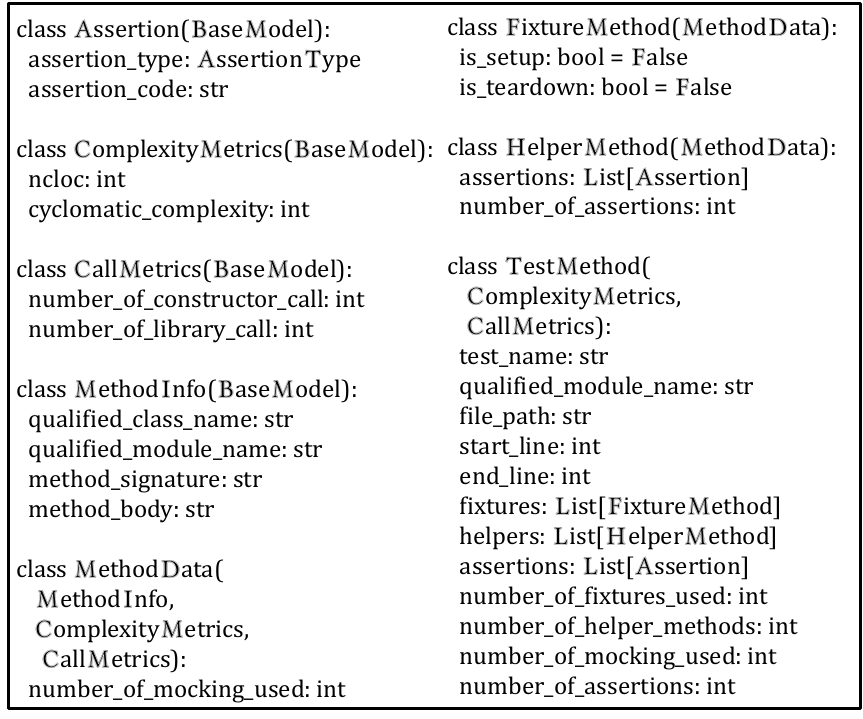}
    \caption{Test complexity code model. \saurabh{move to artifact}}
    \label{fig:test_complexity}
\end{figure}

\begin{figure*}[!htp]
    \centering
    \includegraphics[width=\linewidth]{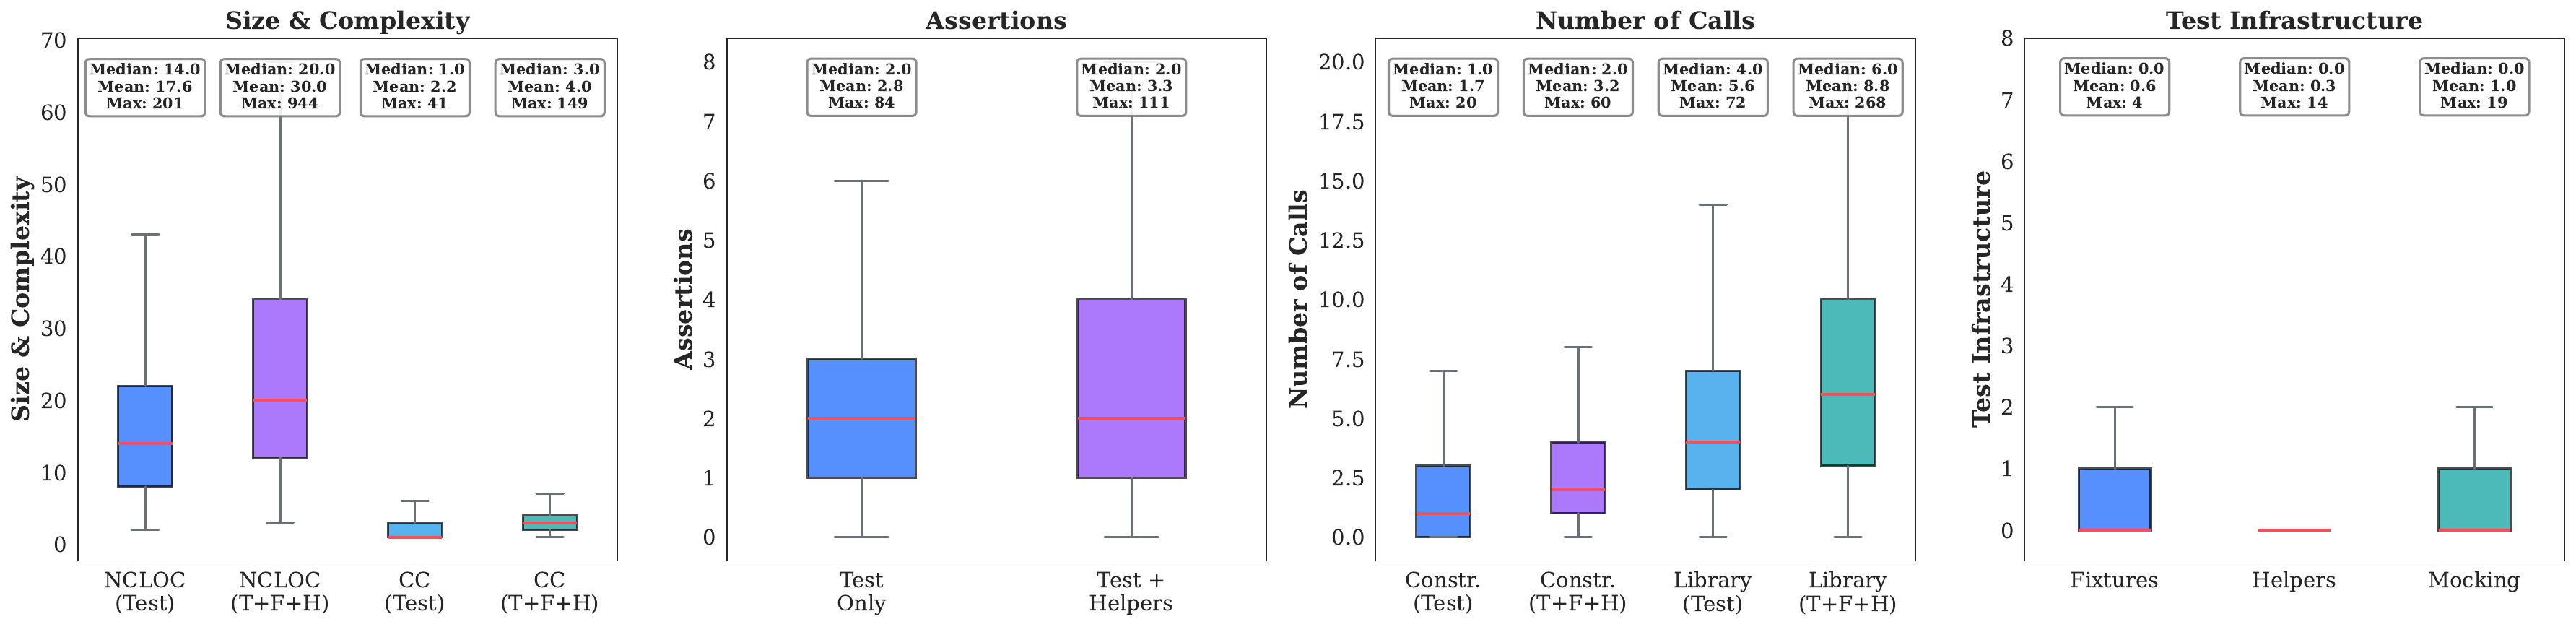}
    \caption{Complexity of agent-related tests.}
    \label{fig:test_complexity}
\end{figure*}
    \begin{pythoncode}
def test_travel_assistant_multimodal_flow(self):
    """Test a comprehensive travel assistant that utilizes multiple modalities:
    1. Create travel itinerary (Text - OpenAI)
    2. Create speech of the itinerary (Speech)
    3. Transcribe speech back to text (Recognition)
    4. Generate destination image (Image)
    5. Analyze image for travel features (Vision)
    6. Create final enhanced travel package (Text - Mistral)
    """
  async def _run_travel_assistant_flow(self):
    # Create tasks dictionary and map paths
    ...
    # 1. Travel Itinerary Creation (OpenAI GPT)
    itinerary_agent = Agent(mission="Create a detailed 3-day travel itinerary",...,)
    itinerary_task = Task(TextTaskInput("Create a 3-day travel itinerary for Rome, Italy. Include major attractions, food recommendations, and transportation tips."),...
    # 2. Speech Synthesis
    speech_agent = self._create_speech_agent()
    speech_task = Task(TextTaskInput("Convert the first day of this itinerary to speech for the traveler"),..)
    # 3. Speech Recognition - OpenAI Whisper
    recognition_agent = Agent(mission="Transcribe the audio guide back to text", ...)
    recognition_task = Task(TextTaskInput("Transcribe this audio accurately"), ...
    # 4. Speech Recognition - Keras Whisper (if model is available)
        keras_recognition_agent = KerasAgent(mission="Transcribe audio using local Whisper model",...)
        keras_recognition_task = Task(TextTaskInput("Transcribe this audio using the local Whisper model"),...
    # 5. Transcription Comparison (only if both transcription tasks exist)
    compare_agent = Agent(mission="Compare the two transcription results",..)
    compare_task = Task(TextTaskInput("Compare these two transcriptions and highlight any differences or quality issues"),...
    # 6. Image Prompt Creation
    img_prompt_agent = self._create_image_prompt_agent()
    img_prompt_task = Task(TextTaskInput("Create a short, specific image generation prompt (under 50 words) for Rome showing the iconic Colosseum")...
    # 7. Destination Image Generation (if Stability AI key is available)
    image_agent = Agent(mission="Generate a visual representation of the destination",...
    # 8. Image Analysis with Vision
    vision_agent = Agent(mission="Analyze the image and identify key landmarks and travel features", ...)
    vision_task = Task(TextTaskInput("Identify the landmarks and notable features in this image that would be relevant for a traveler to Rome")...
    # 9. Final Travel Package (Mistral AI)
    final_agent = Agent(mission="Create an enhanced travel package combining all insights",)
    final_task = Task(TextTaskInput("Create a comprehensive and engaging travel guide for Rome by combining the itinerary, transcription insights, and image analysis")...
    # Create and execute the flow
    flow = Flow(tasks=tasks, map_paths=map_paths, log=True)
    ...
    results = await flow.start(max_workers=3)
    # Validate results
    if not results:
            self.fail("No results were returned from the flow")
    # Validate key outputs
    self.assertIn("itinerary", results, "Itinerary output missing")
    self.assertEqual(results["itinerary"]["type"], "text", "Itinerary should be text type")
    # Check for final package if it exists
    if "final_package" in results:
        self.assertEqual(
            results["final_package"]["type"],"text","Final package should be text type")
    # Validate output files exist
    expected_files = [self.output_files["itinerary"],self.output_files["audio"],self.output_files["image"], self.output_files["travel_guide"]]
    ...
    \end{pythoncode}
